# Supplementary material for: Multimodal, high-dimensional, model-based, Bayesian inverse problems with applications in biomechanics
Source: arXiv:1512.04481 source file (2016-07-21)
Supplement: Supplementary file 1 [file appendixprior.tex]

We consider the following priors for Variational Inference with a single mixture of Gaussians.
\bi
  \item Gaussian prior on $\bs{\Theta}$:
	\\The reduced, latent variables $\bs{\Theta}$ capture the variation of $\bs{\Psi}$ around its mean $\bs{\mu}$. Therefore we assume that the prior of  $\bs{\Theta}$ has zero mean and is uncorrelated. We adapt a multivariate Gaussian prior with
	\be
 	  p(\bt) = \mathcal{N}(\bs{0}, \bs{\Lambda}_0) 
 	  \label{eq:priortheta}
	\ee
	where $\bs{\Lambda}_0 = diag(\lambda_{0,i})$, $i = 1,...,\dth$.
  \item Smoothing regularization prior on $\boldsymbol{\mu}$:
     \\The prior penalizes jumps of neighboring material parameters. The strength of the penalty depends on the hyperparameters $\bs{\Phi}$. 
     Suppose $d_L$ is the total number of jumps or neighboring pairs, then for $j = 1, . . . , d_L$, if $k_j$ and
    $l_j$ denote the corresponding neighboring pair, is follows:
    \be
    p( \mu_{k_j}-\mu_{l_j}| \phi_j)= \sqrt{ \frac{\phi_j}{2\pi}} e^{ -\frac{\phi_{j}}{2} (\mu_{k_j}-\mu_{l_j})^2}
    \label{eq:priormuj}
    \ee
    and for all neighbors summarized:
    \be
    p(\bs{\mu} | \bs{\Phi}) \propto |\bs{\Phi}|^{1/2} e^{-\frac{1}{2} \bs{\mu}^T \bs{L}^T \bs{\Phi} \bs{L} \bs{\mu} }.
    \ee
    As a conjugate prior of the hyperparameters $\bs{\Phi}$ a product of Gamma distributions is chosen:
    \be
      p(\bs{\Phi})=\prod_{j=1}^{d_L} Gamma(a_{\phi},b_{\phi}).
      \label{eq:priorphi}
    \ee	
  \item Prior specification on $\bs{W}$:
	\\To obtain identifiable basis vectors $\bs{w}_i$, where $\bs{w}_i$ are the $i=1,...,\dth$ columns of $\bs{W}$, we require that $\bs{W}$ is orthonormal i.e. $\bs{W}^T \bs{W}=\bs{I}_{\dth}$, where $\bs{I}_{\dth}$ is the $\dth-$dimensional identity matrix. This is equivalent to employing an uniform prior on $\bs{W}$ on the Stiefel manifold $V_{\dth}(\RR^{\dpsi})$ \cite{muirhead_aspects_1982}. 
	In addition we require that $\bs{W}$ is orthogonal to $(\boldsymbol{\hat{y}} - \boldsymbol{y}(\boldsymbol{\mu}))^T \boldsymbol{G}$ to avoid that a basis $\bs{w}_i$ counteracts the optimization of $\bs{\mu}$.	
  \item Gamma prior on $\tau$:
    \\With regards to the noise precision we employ a (conditionally) conjugate Gamma prior:
    \be
      \tau   \sim Gamma(a_0,b_0).  \label{eq:tauPrior}
    \ee
\ei
